# Supplementary material for: Cartesian Products Avoiding Patterns
Source: arXiv:1912.00573 source file (2019-12-02)
Supplement: Supplementary file 1 [file appendix.tex]

\chapter{Supporting Materials}

This would be any supporting material not central to the dissertation.
For example:
\begin{itemize}
\item additional details of methodology and/or data;
\item diagrams of specialized equipment developed.;
\item copies of questionnaires and survey instruments.
\end{itemize}
